# Supplementary material for: Active Third-Person Imitation Learning
Source: arXiv:2312.16365 source file (2023-12-27)
Supplement: Supplementary file 1 [file a16_additional_figures.tex]

\section{Additional Figures}\label{app:additional_figures}
This section presents additional figures corroborating the results of the main paper's experiments (Section~\ref{sec:experiments}). Unless stated otherwise, all plots use the same settings as the ones stated in the experiments section of the main paper. Figure~\ref{fig:correlated_perspectives_point} implies that learning correlations is not harmful even when perspectives are independent. We evaluate this claim in the default specifications of the Point and Reacher environments as defined in Appendix~\ref{app:point:details} and~\ref{app:reacher:details}. Figure~\ref{fig:corr_plain_shaded_bands} shows the training curves for the \textsc{MinProb}, \textsc{MaxProb}, \textsc{UCB} and \textsc{Random} strategies. Indeed, we find the very similar performance of strategies irrespective of correlation learning regarding final reward.

\begin{figure}
  \subcaptionbox{Point}[.5\linewidth]{%
    \includegraphics[width=70mm,scale=0.5]{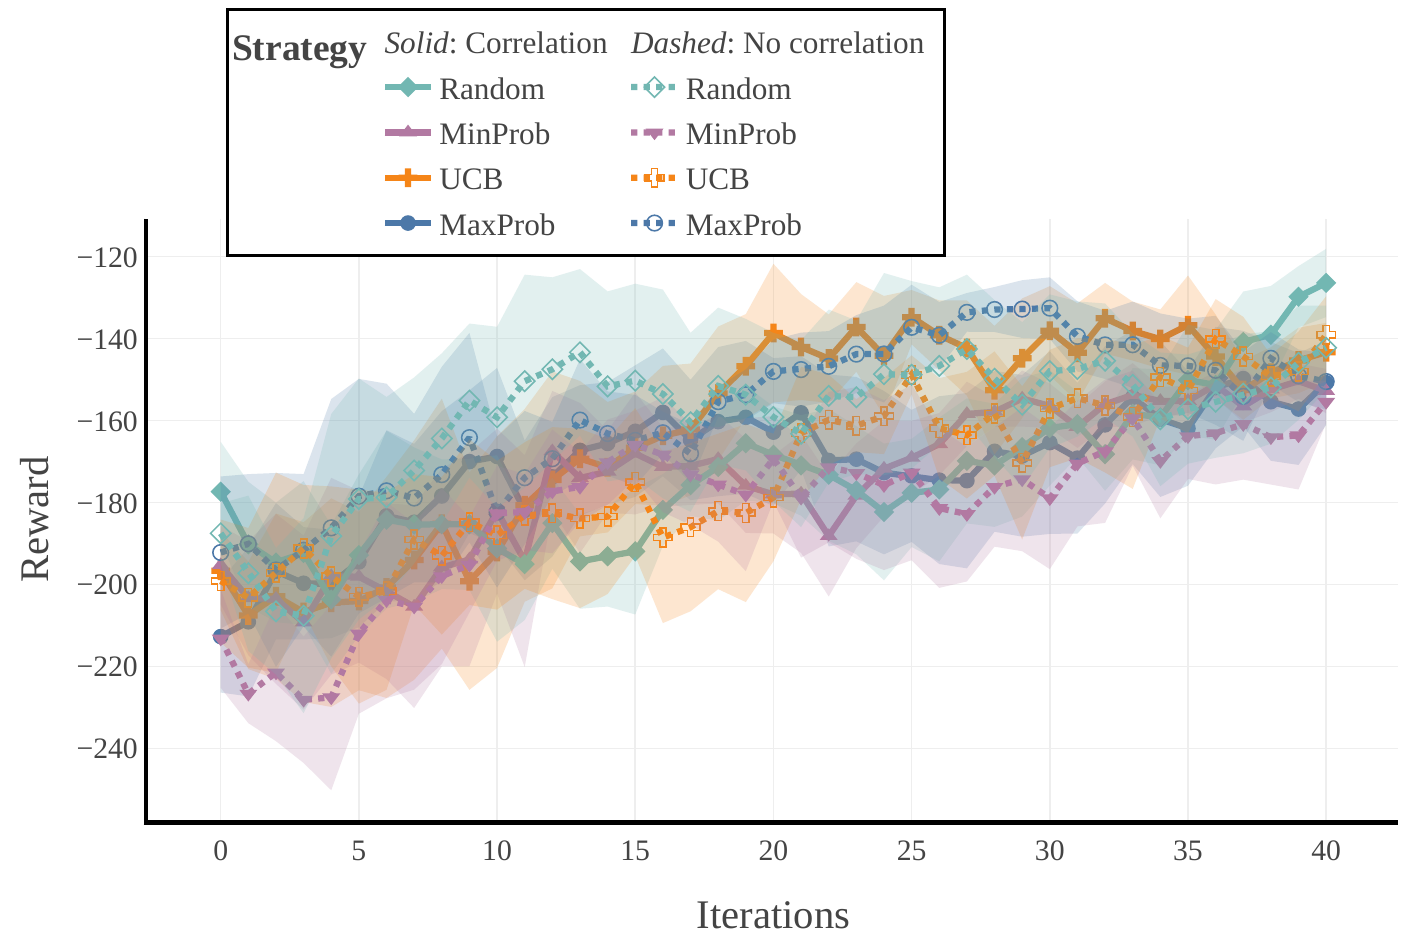}%
  }%
  \hfill
  \subcaptionbox{Reacher}[.5\linewidth]{%
    \includegraphics[width=70mm,scale=0.5]{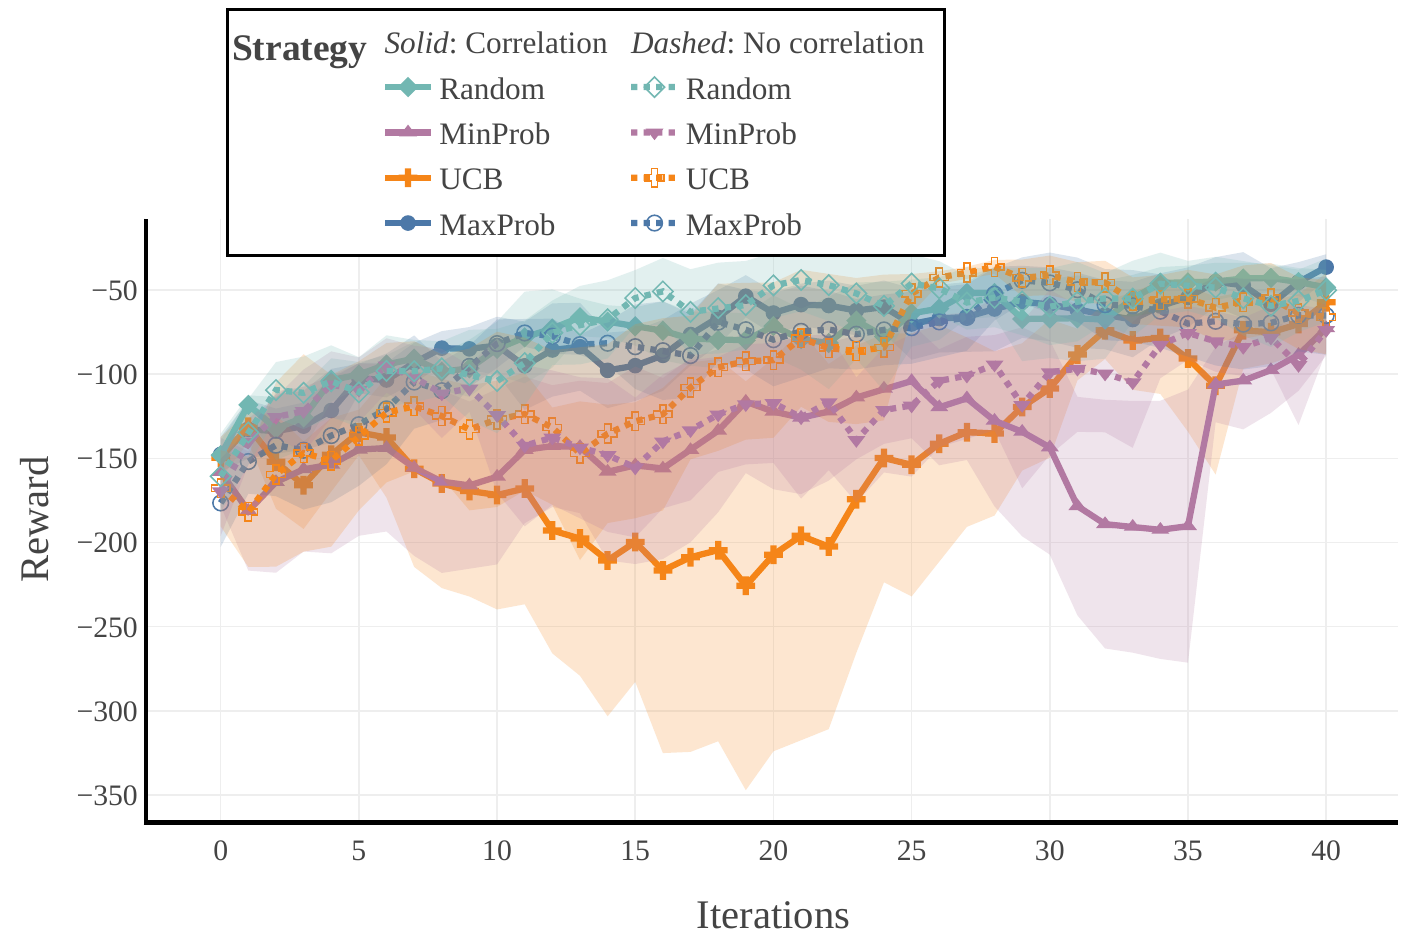}%
  }
    \caption{Effect of correlation learning in the default environment configurations for Point and Reacher. We find no consistent and significant effect on an agent's final performance.}
  \label{fig:corr_plain_shaded_bands}
\end{figure}

One possible conjecture for the superior performance of correlation learning in the Duplicate Point environment may be fewer selections of the no-information perspective. We examine this hypothesis in Figure~\ref{fig:duplicate_point_perspective_bars}. The bar plots show the relative frequency with which perspectives are selected for data generation. Contrary to our working hypothesis, we do not find a substantial difference in selection frequencies for the no-information perspective. However, the plots show that learning correlations produce a better balance between partially informative perspectives. We conjecture that learning about correlations may lead to the agent being able to combine information among perspectives with partial information in a more efficient manner.

\begin{figure}
\label{fig:correlated_perspectives_point:learning_curves_appendix}
\includegraphics[width=70mm,scale=0.5]{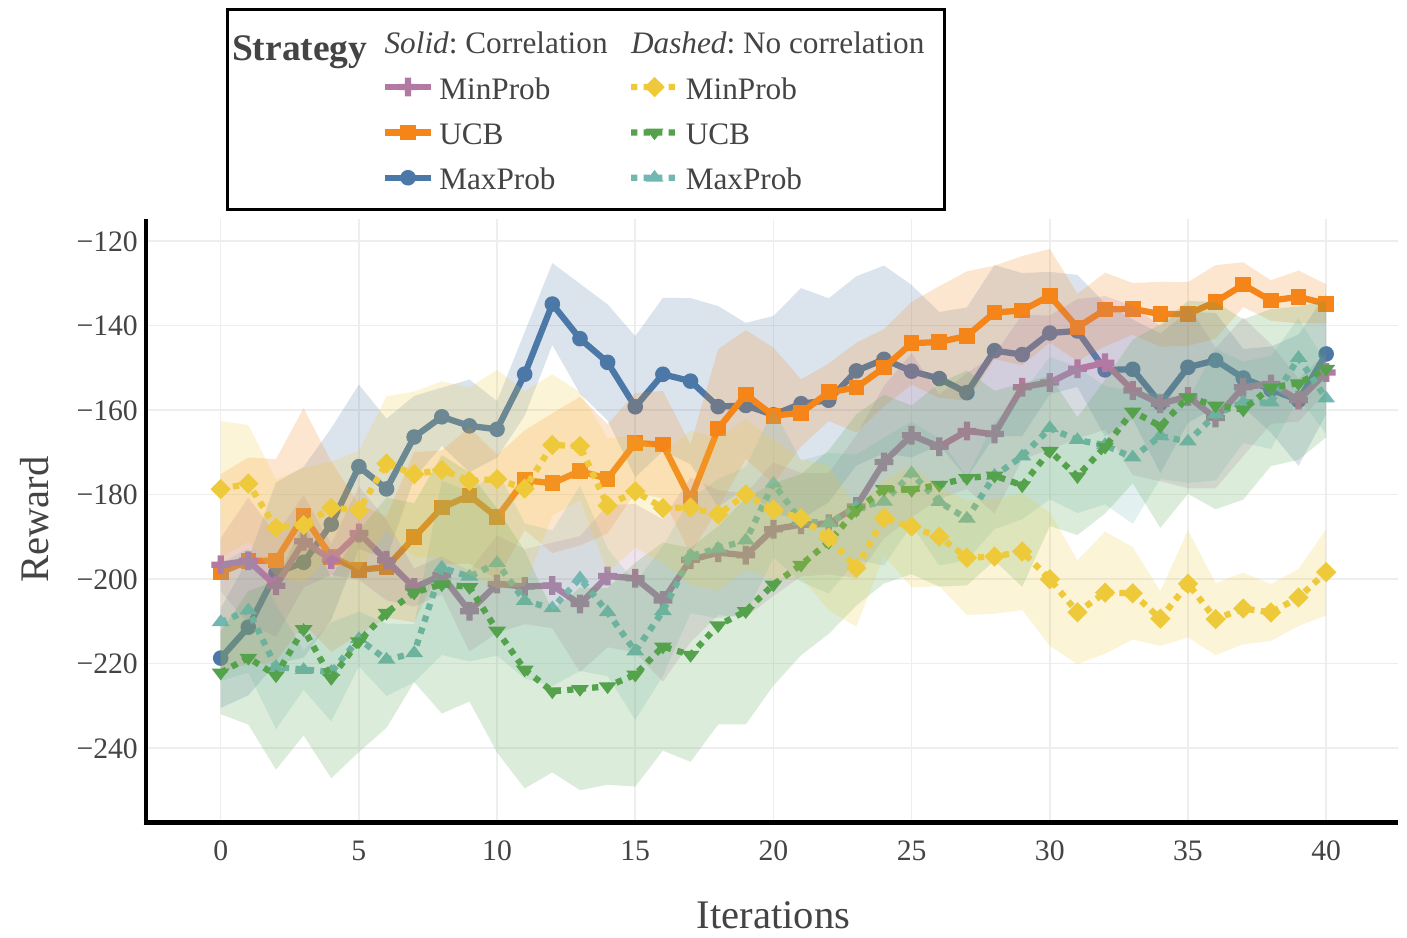}%
  \hfill
\caption{The plot shows the same learning curves for correlation/no correlation learning as the main paper in Figure~\ref{fig:correlated_perspectives_point:learning_curves}.}

\end{figure}

\begin{figure}
  \subcaptionbox{No correlation learning\label{fig:correlated_perspectives_point:bar_no_corr}}[.5\linewidth]{%
    \includegraphics[width=70mm,scale=0.5]{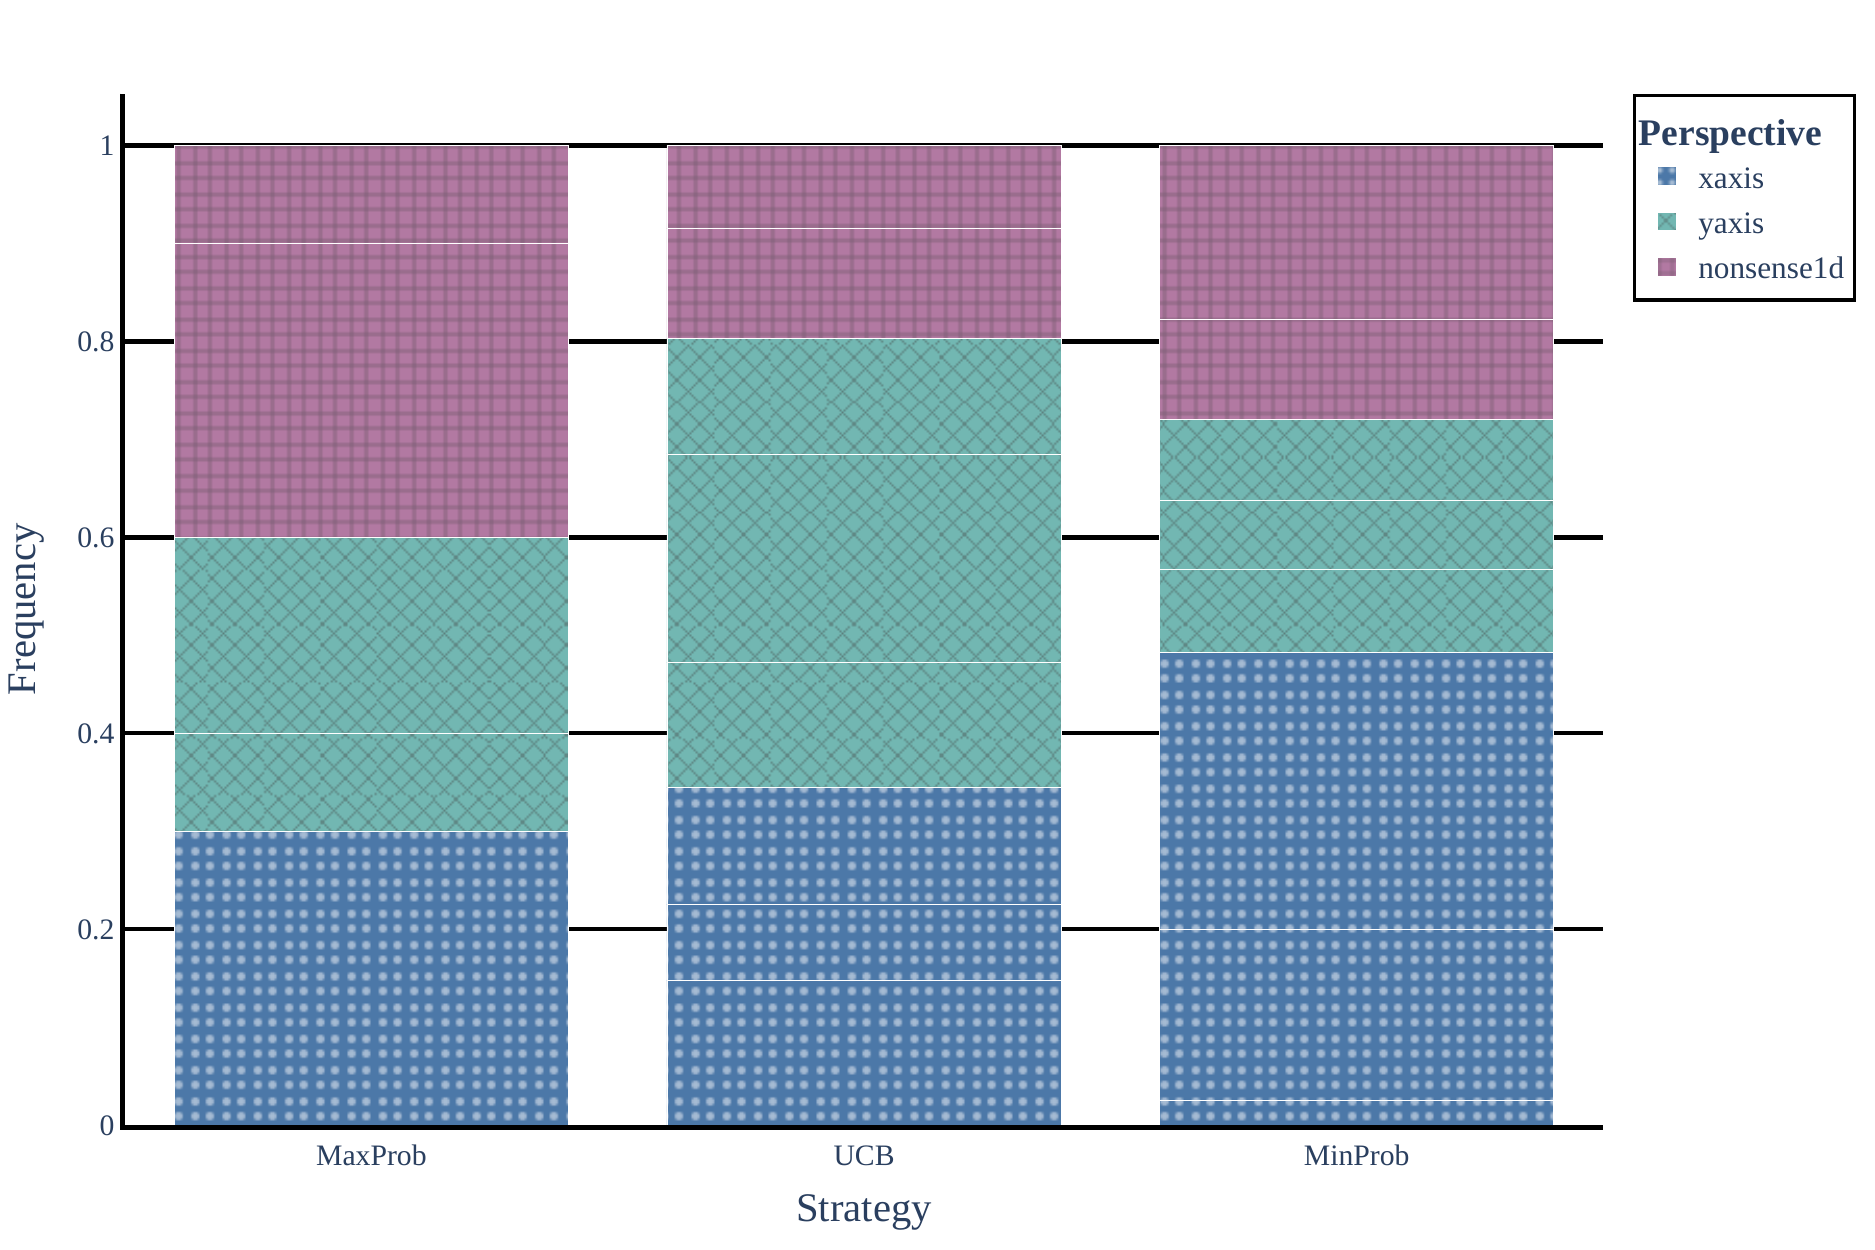}%
  }%
  \hfill
  \subcaptionbox{Correlation learning\label{fig:correlated_perspectives_point:bar_corr}}[.5\linewidth]{%
    \includegraphics[width=70mm,scale=0.5]{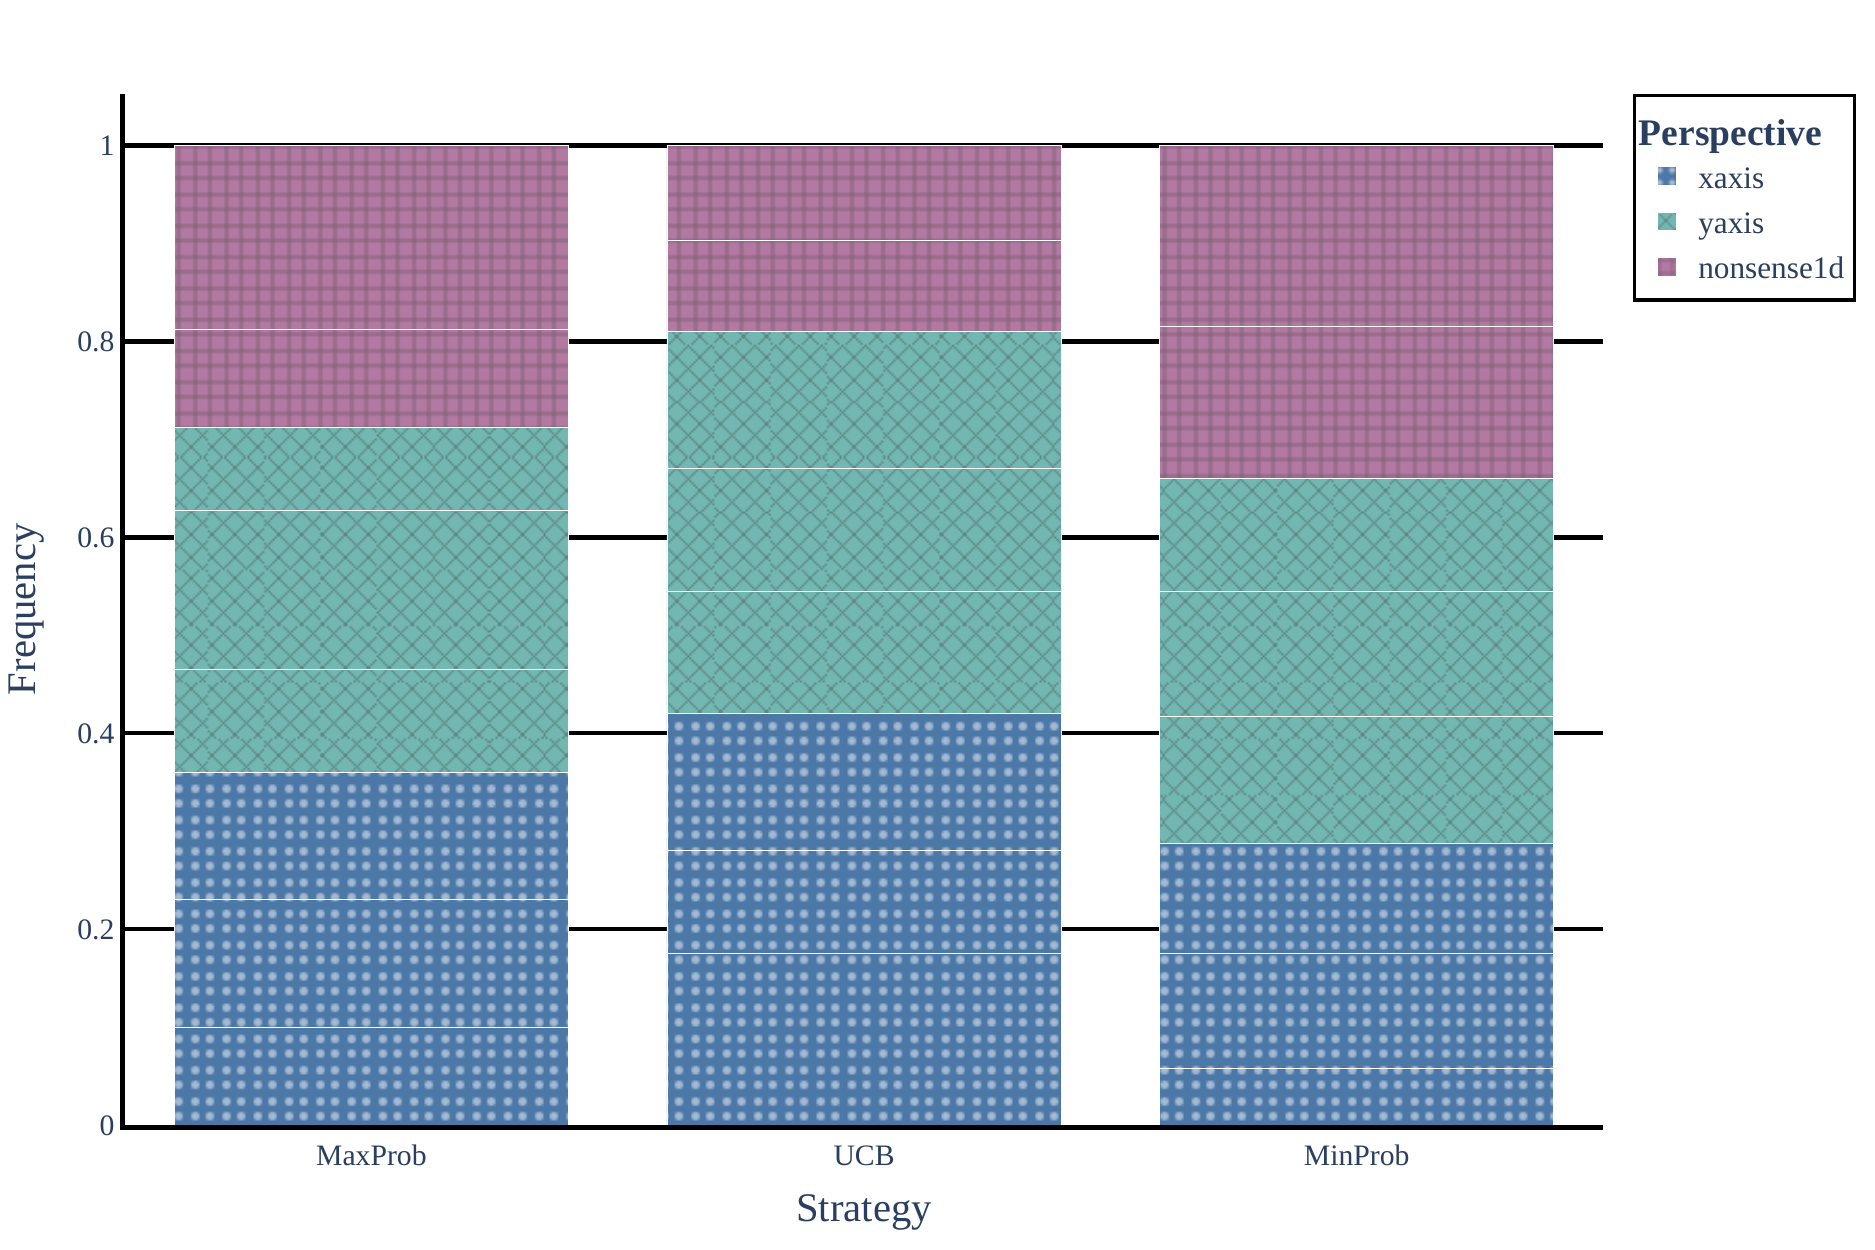}%
  }
    \caption{Selected perspectives for expert data generation on the Duplicate Point environment using all seeds. Learning correlations does not result in a substantially decreased frequency for the no-information perspective except for the \textsc{MaxProb} strategy. However, correlation learning leads to a more balanced selection of perspectives with partial information.}
  \label{fig:duplicate_point_perspective_bars}

\end{figure}

\clearpage
