# Supplementary material for: Active Third-Person Imitation Learning
Source: arXiv:2312.16365 source file (2023-12-27)
Supplement: Supplementary file 2 [file appendix.tex]

\clearpage
\section{Stuff}

\subsection{TODO}
\begin{itemize}
    \item What does the footnote on page 3 bottom left refer to?
\susanna{It refers to the stated formula above $\lambda H(\pi) $ represents the entropy regularisation. We do not use it and there is also a good explanation for it - even in the original paper more than 80 \% of experiments where carried out with $\lambda$=0}
    \item When describing our approach in Section 4: How precisely does this work with the input to the discriminators? Not all perspectives have the same dimensionality.
    \susanna{Yes - I use actually 3 different discriminators based on dimensionality and size (but all are quite similar).
In the text the following is stated \textit{Depending on the perspec-
tives, the discriminator architecture can be slightly different
as we also look into one-dimensional perspectives and adapt
the used image size to the complexity of the environment}}
    \item If there is always the full-information perspective, how do we know that we can effectively extract information from the other perspectives? \susanna{What do you mean? In the experiments I only use the full perspective as baseline, it is not used in any other experiments. In real life I would assume we would just test different experiments and not know if any perspective is better than another.}
    \item What precisely is $\discriminator_v(\Tilde{\omega}^\novice)$?
    \susanna{see 2 points later}
    \item \todo{It is unclear what the legend in the figures means. E.g., what does "partial" mean? What is a "random unlearned policy"? Which perspective is used when talking about "partial information"?}
    \susanna{Is it not clear when reading the text? If not, we can add a description of the baselines in the appendix (currently commented)}
    \item @Susanna: Can you point me to the script with which you produce the plots in the experiments? I am thinking of creating the figures in the right size (then the text will remain readable), putting the legend outside of the plots and make it the plots wider but less high.
    \susanna{\url{https://github.com/stschia/MT_Weinberger/blob/release/run_visualisations.py}, release branch is the one I am working with. I had to rerun some experiments due to a bug. Now we have quite good results for point and reacher. I am still running the experiments for hopper, but unfortunately they did not get better. I would say this is still a result as the perspectives used in the hopper env do not provide much information}
    
    \item $\discriminator(batch^\expert)$ is never explained. By the way, should this still be there? Or should it be based on the notation $\omega$?
    \susanna{You were right this was a bit misleading - I adapted the algorithm. Still it may make sense to remove a bit of complexity and simplify the algorithm}
    \item \susanna{Is the difference between the novice and the novice policy clear?}
    \item \susanna{Paragraph for leveraging information - does that make sense?}
    \item \susanna{Intro: Line 46: Should we write 2 environments if one is only provided in the appendix?}
    \item \susanna{Problem Setting line 19: Should we explain a bit more concise what observations can be}
    \item \susanna{same letter for transition/training algorithm}
    \item \susanna{Text figure 5}
    \item \susanna{related work: add citation}
    \item \susanna{Experiments: Over 20 runs?}
    \item \susanna{Cite observation experiments }
    \item \susanna{Experiment - 2 mal verweis auf Appendix}
    \item \susanna{Additions in Appendix}
    \item \susanna{Graphics for test to find x in UCB}
    \item \susanna{No time for proposed baseline strategy, unfortunately}
\end{itemize}

\section{Done TODOs}

\begin{itemize}
    \item \susanna{Does it make sense to introduce the hopper environment in the paper, but show the experiments later?} \sebastian{Moved.}
    \item In the equation after Figure 3 defining the cross entropy loss. It should be $\discriminator(o_t, o_{t+\Delta}$, right?
    \susanna{as it is stated now it's correct (not sure if you already adapted it). As stated in the text $\hat{y}=\discriminator(o_t, o_{t+\Delta}$ } \sebastian{Adjusted.}
    \item Figure 1: Should we indicate that also the novice can interact with the environment?
\susanna{Would probably make sense yes} \sebastian{Decided to keep it as is.}
\end{itemize}

\paragraph{Including multiple perspectives in one discriminator.}
As the architecture of neural networks is flexible, it is also possible to feed all perspectives in an (adapted) discriminator simultaneously. While this approach has to cope with a more complex neural network and we always need to generate images for all perspectives, it relieves us from the need of training multiple discriminators and from finding defining a strategy to choose the discriminator.

\begin{figure}[h]
  \subcaptionbox*{Point}[.3\linewidth]{%
    \includegraphics[width=\linewidth]{figures/experiments/Point: Combining all perspectives in one discriminator.pdf}%
  }%
  \hfill
  \subcaptionbox*{Reacher}[.3\linewidth]{%
    \includegraphics[width=\linewidth]{figures/experiments/Reacher: Combining all perspectives in one discriminator.pdf}%
  }
  \hfill
    \subcaptionbox*{Hopper}[.3\linewidth]{%
    \includegraphics[width=\linewidth]{figures/experiments/Hopper: Combining all perspectives in one discriminator.pdf}%
  }
    \caption{Comparison to an all-perspective discriminator}
  \label{fig:exp5}
  
\end{figure}

\sebastian{Should we consider a zero-imputation strategy in which the perspective selection is just another possible action as a baseline?}
